# Supplementary material for: Cross-Lingual Ability of Multilingual BERT: An Empirical Study
Source: arXiv:1912.07840 source file (2020-02-15)
Supplement: Supplementary file 1 [file Appendix.tex]

% \section{Appendix}


% \subsection{Further discussions on Structural Similarity}

% In the main text, we defined structural similarity as all the properties of a language that is invariant to the script of the language, like morphology, word-ordering, word-frequency, etc.. Here, we analyze 2 sub-components of structural similarity -- word-ordering similarity and word-frequency (Unigram frequency) similarity to understand the concept of structural similarity better. 

% \subsubsection{Word-Ordering Similarity}

% % \begin{table*}[!htbp]
% % \small
% % \centering
% % \begin{threeparttable}
% % %\caption{The Effect of Word-Piece Overlap and of Structural Similarity.}
% % \begin{tabular*}{\textwidth}{ c @{\extracolsep{\fill}} c c c c c} 
% % \toprule
% % % \multicolumn{3}{c}{} & \multicolumn{2}{c}{\textbf{XNLI}} &  \multicolumn{1}{c}{\textbf{NER}}  \\
% % % \cmidrule(l){4-5} \cmidrule(l){6-6}
% % \textbf{B-BERT} & \textbf{Train} & \textbf{Test} & \textbf{XNLI (acc)}  &  \textbf{NER (Span F1-Score)}  \\
% % \midrule
% % enfake-es & enfake & es & 70.9 \\
% % % enfake-es-permute-0.25  & enfake & es & 67.5 \\
% % enfake-es-permute-0.50  & enfake & es & 64.6\\
% % enfake-es-permute-1.00  & enfake & es & 58.9\\
% % \midrule
% % enfake-hi & enfake & hi & 59.6  \\
% % % enfake-hi-permute-0.25  & enfake & hi & 47.0\\
% % enfake-hi-permute-0.50 & enfake & hi & 48.8 \\
% % enfake-hi-permute-1.00 & enfake & hi & 46.5 \\
% % \midrule
% % enfake-ru & enfake & ru & 65.7 \\
% % % enfake-ru-permute-0.25 & enfake & ru &\\
% % enfake-ru-permute-0.50 & enfake & ru & 56.5\\
% % enfake-ru-permute-1.00 & enfake & ru & 57.8\\
% % \bottomrule
% % \end{tabular*}
% % \vspace*{-6px}
% %     \caption{
% %     %\begin{tablenotes}
% %     \small
% %     {\bf Contribution of Word-Ordering similarity:} We study the importance of word-order similarity by comparing the performance of XNLI and NER with a certain percent of word-order similarity. FOr a certain percent $p$, we permute the sentence in two ways, (1) SWAP: randomly swap two words in a sentence for $p * (L - 1)$ times, where $L$ is the number of words in the sentence, and (2) SHUFFLE: randomly shuffle $p * L$ words in the sentence. FakeEnglish $\to$ Spanish has a significant decrease in performance from $50\%$ to $100\%$, indicating that some order similarity still preserves even after a $50\%$ of shuffle.}
% % \label{tbl:LinguisticFeature}
% % \end{threeparttable}
% % \vspace*{-6px}
% % \end{table*}

% Words are ordered differently between languages. For example, English has a Subject-Verb-Object order, while Hindi has a Subject-Object-Verb order. We analyze whether similarity in how words are ordered affects learning cross-lingual transferability. We study the effect of word-ordering similarity -- one component of structural similarity -- by destroying the word-ordering structure by shuffling some percentage of random words in sentences during pretraining. We shuffle both source (fake-English) and target language (permuting any one of them would also be sufficient).  This way, the similarity of word-ordering is hidden from B-BERT. We model how much we permute each sentence, for example, when the sentence is 100\% permuted, each sentence can be treated as a Bag of Words. For each word, the words that appear in its context (other words in the sentence) is not changed. 

% Note that during fine-tuning on source language (and testing on target language), we do not permute, as the cross-lingual ability is gained only during the pretraining process.

% From Table~\ref{tbl:Word-order}, we can see that the performance drops significantly when we destroy word-order similarity. However, the cross-lingual performance is still quite good, which indicates that there are other components of structural similarity, which could contribute to the cross-lingual ability of \BBERT.
 
% \begin{table*}[!htbp]
% \small
% \centering
% \begin{threeparttable}
% \begin{tabular*}{\textwidth}{ c @{\extracolsep{\fill}} c c c c c} 
% \toprule
% \textbf{B-BERT} & \textbf{Train} & \textbf{Test} & \textbf{XNLI (acc)}  &  \textbf{NER (Span F1-Score)}  \\
% \midrule
% enfake-es & enfake & es & 70.9 & 62.6 ($\pm$1.6)\\
% enfake-es-permute-0.25  & enfake & es & 68.9 & 42.3 ($\pm$ 0.6)\\
% enfake-es-permute-0.50  & enfake & es & 65.5 & 41.3 ($\pm$3.8)\\
% enfake-es-permute-1.00  & enfake & es & 62.5 & 39.4 ($\pm$1.5) \\
% \midrule
% enfake-hi & enfake & hi & 59.6 & 62.9 ($\pm$0.7) \\
% enfake-hi-permute-0.25  & enfake & hi & 51.4 & 24.8 ($\pm$2.0)\\
% enfake-hi-permute-0.50 & enfake & hi & 48.3 & 8.7 ($\pm$1.9)\\
% enfake-hi-permute-1.00 & enfake & hi & 43.1 & 2.9 ($\pm$1.9)\\
% \midrule
% enfake-ru & enfake & ru & 65.7 & 54.2 ($\pm$0.7) \\
% enfake-ru-permute-0.25 & enfake & ru & 63.6 & 23.6 ($\pm$2.3)  \\
% enfake-ru-permute-0.50 & enfake & ru & 59.7 & 16.3 ($\pm$0.4)\\
% enfake-ru-permute-1.00 & enfake & ru & 53.6 &16.3 ($\pm$0.9) \\
% \bottomrule
% \end{tabular*}
% \vspace*{-6px}
%     \caption{
%     %\begin{tablenotes}
%     \small
%     {\bf Contribution of Word-Ordering similarity:} We study the importance of word-order similarity by analysing the performance of XNLI and NER when some percent of word-order similarity is destroyed. For a certain percent $p$, we randomly shuffle $p * L$ words in the sentence, where $L$ is the number of total number of words in that sentence. For example, enfake-es-permute-0.25 indicates that in each sentence a random 25\% of words are shuffled and enfake-es-permute-1.00 indicates every word in the sentence is randomly shuffled, similarly for others. We can see that word-order similarity is quite important, however there must be other components of structural similarity that could contribute for the cross-lingual ability, as the the performance of enfake-es-permute-1.00 is still pretty good.}
% \label{tbl:Word-order}
% \end{threeparttable}
% \vspace*{-6px}
% \end{table*}






% \subsubsection{Word-frequency Similarity}

% Here, we study whether only word frequency allows for good cross-lingual representations -- no, it is not much useful. We collect the frequency of words in the target language and generate a new monolingual corpus by sampling words based on the frequency, i.e., each sentence is a set of random words sampled from the same unigram frequency as the original target language. The only information about target language BERT has is its unigram frequency and sub-word level information. We train \BBERT using Fake-English and this newly generated target corpus. From Table~\ref{tbl:UnigramFrequency}, we can see that the performance is very low, although non-trivial (random performance is 33.33\%). Therefore, unigram frequencies alone don't contain enough information for cross-lingual learning (bi-gram or tri-gram frequencies might be useful).


% \begin{table*}[!htbp]
% \vspace*{-5px}
% \small
% \centering
% \begin{threeparttable}
% \begin{tabular*}{\textwidth}{ c @{\extracolsep{\fill}} c c c c c}
% \toprule
% \textbf{B-BERT} & \textbf{Train} & \textbf{Test} & \textbf{XNLI (acc)}  &  \textbf{NER (Span F1-Score)}  \\
% \midrule
% enfake-es & enfake & es & 70.9 & 62.6 ($\pm$1.6)\\
% enfake-es-freq  & enfake & es & 35.4 & 15.0($\pm$ 1.1)\\
% \midrule
% enfake-hi & enfake & hi & 59.6 & 62.9 ($\pm$0.7) \\
% enfake-hi-freq & enfake & hi & 36.3 & 1.2 ($\pm$0.9)\\
% \midrule
% enfake-ru & enfake & ru & 65.7 & 54.2 ($\pm$0.7)\\
% enfake-ru-freq & enfake & ru & 34.4 & 5.7 ($\pm$0.5)\\
% \bottomrule
% \end{tabular*}
% \vspace*{-6px}
%     \caption{
%     %\begin{tablenotes}
%     \small
%     {\bf Cross-lingual ability from only Unigram frequency:} We study if only unigram frequency is useful for cross-lingual transfer. enfake-es-freq indicates \BBERT trained with Fake-English and the new created corpus, where each sentence is a set of random words sampled from the same unigram distribution as es. The results show that only unigram frequency is not enough for a reasonable cross-lingual performance.}
% \label{tbl:UnigramFrequency}
% \end{threeparttable}
% \vspace*{-6px}
% \end{table*}






% \subsection{Further discussions on Architecture }

% \subsubsection{Multilingual BERT}
% All the experiments in the main text are conducted on Bilingual BERT. However, the results hold even for the multilingual case; to further illustrate this, we experiment on four language BERT (en, es, hi, ru). From Table~\ref{tbl:multilingual}, we can see that the performance on XNLI is comparable even with just 15\% of parameters, and just 1, 3 attention heads when the depth is good enough, which is in agreement with our observations in the main text.

% Also, currently, there is a lot of interest in reducing the size of BERT~\citep{anonymous2020reweighted}, using various pruning techniques. Our analysis shows that we can get comparable performance by maintaining (or increasing) depth. Indeed, by changing the number of parameters from 132.78M to 20.05M (approx 85\% less) by reducing only the hidden layer sizes, the English performance drops only from 79.0 to 75.0 (about 4\%), which is comparable to the drop in MNLI performance of~\citep{anonymous2020reweighted}, where the performance drops by -4.7\% for 88.4\% reduction of parameters (English XNLI is similar to MNLI). We believe that these pruning techniques could be combined with the insights from the paper to get much better results. 


% \begin{table*}[!htbp]
% \vspace*{-5px}
% \small
% \centering
% \begin{threeparttable}
% % \caption{Architecture - Contribution of Multi-head Attention }
% \begin{tabular*}{\textwidth}{ c @{\extracolsep{\fill}} c c c c c c } 
% \toprule
% \multicolumn{3}{c}{} & \multicolumn{4}{c}{\textbf{XNLI}} \\
% \cmidrule{4-7}
% \textbf{Parameters (in Millions)}  & \textbf{Depth} & \textbf{Multi-head Attention} & \textbf{en} & \textbf{es} & \textbf{hi} & \textbf{ru}\\ 
% \midrule
% 132.78 (100\%) & 12 & 12 & 79.0 & 70.0 & 50.7 & 65.2 \\
% \midrule
% 20.05 (15.1\%)  & 16 & 1 & 74.1 & 63.2 &	49.6 & 58.9\\
% 20.05 (15.1\%)  & 16 & 3 & 75.0 & 65.3 & 51.1 & 60.3 \\
% \midrule
% 24.20 (18.23\%) & 24 & 1 & 75.0 & 64.5 & 48.3 & 58.6 \\
% 24.20 (18.23\%) & 24 & 3 & 75.7 & 65.5 & 48.9 & 60.2 \\
% \midrule
% 30.43 (22.92\%) & 36 & 1 & 75.2& 66.5& 47.1 & 60.3\\
% 30.43 (22.92\%) & 36 & 3 & 76.0 &	64.8 &	47.8& 59.8\\ 
% \bottomrule
% \end{tabular*} 
% \vspace*{-6px}
% \caption{
%     \small
%     {\bf Significantly smaller multilingual BERT:} We show that the insights derived from bilingual BERT is valid even in the case of multilingual BERT (4 language BERT). Further, we also show that with enough depth, we only need a fewer number of parameters and attention heads to get comparable results.}
% \label{tbl:multilingual}
% \end{threeparttable}
% \vspace*{-8px}
% \end{table*}



% \subsubsection{Number of parameters}

% Here we show more results on the effect of the number of parameters to get more insights on the threshold on the number of parameters. The experimental setting was similar to that of table~\ref{tbl:NumberOfParameters}. 

% From table~\ref{tbl:NumberOfParametersfull}, we can notice a drastic change in the performance of Russian when the number of parameters is decreased from  11.83M to 7.23M, so we can consider this range to be the required minimum number of parameters, at least for the 12 layer and 12 attention heads situation.


% \begin{table*}[!htbp]
% \vspace*{-8px}
% \small
% \centering
% \begin{threeparttable}
% \begin{tabular*}{\textwidth}{ c@{\extracolsep{\fill}} c c c c c} 
% \toprule
% \multicolumn{3}{c}{} & \multicolumn{3}{c}{\textbf{XNLI}}\\
% \cmidrule{4-6}
% \textbf{Parameters (in Millions)} & \textbf{Depth} & \textbf{Multi-head Attention} & \textbf{Fake-English} & \textbf{Russian} & \textbf{$\Delta$}\\ 
% \midrule
% 4.23 & 12 & 12 & 65.5 & 46.6 & 18.9\\
% \textbf{7.23} & \textbf{12} & \textbf{12} & 68.5 & \textbf{49.9} & 18.6 \\
% \textbf{11.83} & \textbf{12} & \textbf{12} & 71.3 & \textbf{56.3} & 15.0 \\
% 15.71 & 12 & 12 & 72.9 & 58.2 & 14.7\\ 
% 23.03 & 12 & 12 &  74.8 & 60.9 & 13.9 \\
% 29.65 & 12 & 12  & 76.6 &  61.4 &  15.2 \\
% 44.89 & 12 & 12  & 78.2 & 64.0 & 14.2 \\
% 89.03 & 12 & 12  & 78.6 & 64.1 & 14.5 \\
% 283.11 & 12 & 12  & 79.6 & 65.4 & 14.2 \\
% \midrule 
% 132.78 & 12 & 12 & 79.0  &  65.7  & 13.3 \\
% \midrule
% \bottomrule
% \end{tabular*}
% \vspace*{-6px}
% \caption{
%     \small
%     {\bf The Effect of Total Number of Parameters:} We study the effect of the total number of Parameters of \BBERT on the performance of Fake-English and Russian language on XNLI data. We fix both the number of depth and number of attention heads of \BBERT and vary the total number of parameters by changing the size of hidden and intermediate units. The difference between the performance on Fake-English and Russian($\Delta$) is our measure of cross-lingual ability. We can see that there is a drastic change in performance when we reduce the number of parameters from 11.83M to 7.23M, so this is threshold for kind of a number of parameters.}
% \label{tbl:NumberOfParametersfull}

% \end{threeparttable}
% \vspace*{-8px}
% \end{table*}





% % \subsection{Same language Experiments}

% % \begin{table*}[htbp]
% % \centering
% % \begin{threeparttable}
% % \caption{Misc - Same Language Sentence pair Experiment}
% % \label{tbl:SameLanguage}
% % \begin{tabular}{ c c c c c c c} 
% % \toprule
% % \multicolumn{3}{c}{} & \multicolumn{2}{c}{\textbf{XNLI}} & \multicolumn{2}{c}{\textbf{NER}}\\
% % \cmidrule(l){4-5} \cmidrule(l){6-7}
% % \textbf{BERT} & \textbf{Train} & \textbf{Test} & \textbf{Anything}   & \textbf{Same-lang-pair}  & \textbf{Anything}   & \textbf{Same-lang-pair}  \\
% % \midrule
% % \multirow{2}{*}{enfake-es} & \multirow{2}{*}{enfake} &  enfake & 78.5 & 79.0 &  &\\ 
% % & & es & 70.9 & 73.0  &  & \\
% % \midrule
% % \multirow{2}{*}{enfake-hi} & \multirow{2}{*}{enfake} &  enfake & 79.3 & 80.0 &  & \\ 
% % & & hi & 59.6 & 58.0 &  & \\
% % \midrule
% % \multirow{2}{*}{enfake-ru} & \multirow{2}{*}{enfake} &  enfake & 79.0 & 79.1  &    & \\ 
% % & & ru & 65.7 & 67.5 &   &  \\
% % \bottomrule
% % \end{tabular}
% %     \begin{tablenotes}
% %     \small
% %     \item  Anything -- SENT1 and SENT2 can be any language independently
% %     \item Same-lang-pair -- SENT1 and SENT2 must be same language
% %     \end{tablenotes}
% % \end{threeparttable}
% % \end{table*}







% % \subsection{Intrinsic Study}

% % \begin{table*}[!htbp]
% % \centering
% % \begin{threeparttable}
% % \caption{Similarity between Parallel Sentences - Intrinsic Measure}
% % \label{tbl:Intrinsic}
% % \begin{tabular}{ c c c c c c } 
% % \toprule
% % \textbf{Language-1} & \textbf{Language-2} & \textbf{Metric} & \textbf{BERT} & 
% % \textbf{\textcolor{red}{Flair}} & \textbf{Deep Word2Vec} \\
% % \midrule
% % \multirow{2}{*}{enfake} & \multirow{2}{*}{en} & Top-1 & 98.2 &  79.1 & 0.1 \\
% %  &  & Top-3 & 99.8  & 86.3 & 0.6 \\
% % \midrule
% % \multirow{2}{*}{enfake} & \multirow{2}{*}{es} &  Top-1 & 76.5 & 2.0 & \\
% %  &  & Top-3  & 85.5 & 4.7 & \\
% % \midrule
% % \multirow{2}{*}{enfake} & \multirow{2}{*}{hi} & Top-1 & 34.4 &  0.1 \\
% %  &  & Top-3  &  46.2 & 0.8 \\
% % \midrule
% % \multirow{2}{*}{enfake} & \multirow{2}{*}{ru} & Top-1 & 63.6 & 1.6 & \\
% %  &  & Top-3 & 79.0 & 3.8 \\
% % \bottomrule
% % \end{tabular}
% %     \begin{tablenotes}
% %     \small
% %     \item 
% %     \end{tablenotes}
% % \end{threeparttable}
% % \end{table*}









% % \subsection{Random Shuffling}
